# Supplementary material for: Reducing the Deployment-Time Inference Control Costs of Deep Reinforcement Learning Agents via an Asymmetric Architecture
Source: arXiv:2105.14471 source file (2021-05-30)
Supplement: Supplementary file 1 [file cross_referencing.tex]

% Notes:
% If the labels in the supplementary material have changed, please clear cached files and recompile.
%
% References:
% https://www.overleaf.com/learn/how-to/Cross_referencing_with_the_xr_package_in_Overleaf
% https://texfaq.org/FAQ-extref
% https://tex.stackexchange.com/a/248501

%%%%%%%%%%%%%%%%%%%%%%%%%%%%%%%%%%%%%%%%%%%%%%%%%%%%%%%%%%%%%%%%%%%%%%%%%%%%%%%
% # Use Packages
%%%%%%%%%%%%%%%%%%%%%%%%%%%%%%%%%%%%%%%%%%%%%%%%%%%%%%%%%%%%%%%%%%%%%%%%%%%%%%%

% ## zref – A new reference scheme for LATEX
%
% This package provides extensible referencing system.
%
% See the documentation for more information.
%
% CTAN: https://ctan.org/pkg/zref

\usepackage[user,xr]{zref}

%%%%%%%%%%%%%%%%%%%%%%%%%%%%%%%%%%%%%%%%%%%%%%%%%%%%%%%%%%%%%%%%%%%%%%%%%%%%%%%
% # Customize
%%%%%%%%%%%%%%%%%%%%%%%%%%%%%%%%%%%%%%%%%%%%%%%%%%%%%%%%%%%%%%%%%%%%%%%%%%%%%%%

% ## Customize zref

\ifdef{\zxrsetup}{
    % Package `zref` is used

    % Make external references available to \ref{}

    % \zxrsetup{
    %     tozreflabel=false,
    %     toltxlabel=true,
    % }

    % Check whether the draft mode is on
    \ifbool{draftmode}{
        % Draft mode is on
    }{
        % Draft mode is off

        % Check whether the external file `main.tex` and `sup.tex` exist
        %
        % References:
        % https://tex.stackexchange.com/a/98205

        \IfFileExists{main.tex}{
            % The file `main.tex` exists

            \IfFileExists{sup.tex}{
                % The file `sup.tex` exists

                % Load external references from `main.tex` and make the labels able to be referenced with prefix "main:"
                \zexternaldocument*[main:]{main}

                % Load external references from `sup.tex` and make the labels able to be referenced with prefix "sup:"
                \zexternaldocument*[sup:]{sup}

            }{
                % The file `sup.tex` doesn't exist
            }

        }{
            % The file `main.tex` doesn't exist
        }

    }

}{
    % Package `zref` is not used
}
