# Supplementary material for: Reducing the Deployment-Time Inference Control Costs of Deep Reinforcement Learning Agents via an Asymmetric Architecture
Source: arXiv:2105.14471 source file (2021-05-30)
Supplement: Supplementary file 2 [file floats.tex]

% References:
% https://en.wikibooks.org/wiki/LaTeX/Floats,_Figures_and_Captions

%%%%%%%%%%%%%%%%%%%%%%%%%%%%%%%%%%%%%%%%%%%%%%%%%%%%%%%%%%%%%%%%%%%%%%%%%%%%%%%
% # Use Packages
%%%%%%%%%%%%%%%%%%%%%%%%%%%%%%%%%%%%%%%%%%%%%%%%%%%%%%%%%%%%%%%%%%%%%%%%%%%%%%%

% ## afterpage – Execute command after the next page break
%
% This package can be used to move floats to the next page.
%
% ### Usage
%
% Surround the float with `\afterpage{<float>}` to make it appear after the current page.
%
% ### Examples
%
% Move the figure one column (or one page) later after the current column:
% ```latex
% \afterpage{
%     \begin{figure}[t]
%         \centering
%         \fbox{
%             \rule{0pt}{50pt}
%             \rule{50pt}{0pt}
%         }
%         \caption{A figure.}
%         \label{fig:figure}
%     \end{figure}
% }
% ```
%
% CTAN: https://ctan.org/pkg/afterpage

\usepackage{afterpage}

%------------------------------------------------------------------------------

% ## caption – Customising captions in floating environments
%
% This package is used for reducing vertical spacing after floats.
%
% CTAN: https://ctan.org/pkg/caption

\usepackage[
    labelfont=bf
]{caption}

%------------------------------------------------------------------------------

% ## graphicx – Enhanced support for graphics
%
% This package allows you to import external graphics.
%
% ### Usage
%
% Insert the graphic with the command:
% ```latex
% \includegraphics[<options>]{<file>}
% ```
% The most common used option is `width=<value>`, which scales the graphic to this value.
%
% ### Examples
%
% To insert an image `image.png`, add:
% ```latex
% \includegraphics[width=.3\linewidth]{image.png}
% ```
% `width=.3\linewidth` scales the graphic down to 0.3 relative to the width of a line. Scaling down is usually used in subfigures.
%
% CTAN: https://ctan.org/pkg/graphicx
% Reference: https://en.wikibooks.org/wiki/LaTeX/Importing_Graphics

\usepackage{graphicx}

\usepackage[
    labelformat=simple
]{subcaption}

\ifdef{\captionsetup}{
    % Package `caption` is used

    % Customize figure environment
    \captionsetup[figure]{
        % Font size option
        font=small,
        % Vertical space between float and caption
        skip=0.5em
    }

    % Customize table environment
    \captionsetup[table]{
        % Font size options
        font=small,
        % Vertical space between float and caption
        % skip=0.5em
    }

    % Customize subcaption environment
    \ifdef{\subcaption}{
        % Package `subcaption` is used

        \captionsetup[sub]{
            % Font size options
            font=small,
            % Vertical space between sub-float and sub-caption
            skip=0.5ex
        }

    }{
        % Package `subcaption` is not used
    }

    % Customize subfig environment
    \ifdef{\subfloat}{
        % Package `subfig` is used

        \captionsetup[subfloat]{
            % Font size option
            font=small,
            % Vertical space between sub-float and sub-caption
            % captionskip=1ex
            % Vertical space between float and caption
            % nearskip=1ex
        }

    }{
        % Package `subfig` is not used
    }

}{
    % Package `caption` is not used
}

% ## Customize subcaption

\ifdef{\thesubfigure}{
    % Command `thesubfigure` exists

    % Change referencing format from 1a to 1 (a)
    %
    % Note:
    % To use this modification, please add the option `labelformat=simple` to the package `subcaption` or the options `caption=false,labelformat=simple` to the package `subfig`.
    \renewcommand{\thesubfigure}{~(\alph{subfigure})}

}{
    % Command `thesubfigure` doesn't exist
}
