# Supplementary material for: Reducing the Deployment-Time Inference Control Costs of Deep Reinforcement Learning Agents via an Asymmetric Architecture
Source: arXiv:2105.14471 source file (2021-05-30)
Supplement: Supplementary file 3 [file hyperlinks.tex]

% References:
% https://en.wikibooks.org/wiki/LaTeX/Hyperlinks

%%%%%%%%%%%%%%%%%%%%%%%%%%%%%%%%%%%%%%%%%%%%%%%%%%%%%%%%%%%%%%%%%%%%%%%%%%%%%%%
% # Use Packages
%%%%%%%%%%%%%%%%%%%%%%%%%%%%%%%%%%%%%%%%%%%%%%%%%%%%%%%%%%%%%%%%%%%%%%%%%%%%%%%

\ifbool{draftmode}{
    % Draft mode is on

    % ## hyperref – Extensive support for hypertext in LATEX
    %
    % This package allows you to write commands to produce hypertext links.
    %
    % ### Usage
    %
    % Some common commands include:
    % ```latex
    % \href{<URL>}{<text>}
    % \url{<URL>}
    % \hyperref[<label>]{<text>}
    % ```
    %
    % ### Examples
    %
    % Add the following line in document:
    % ```latex
    % \href{https://google.com}{Google}
    % \url{https://google.com}
    % Section~\hyperref[sec:intro]{\ref*{sec:intro}}
    % ```
    %
    % ### Options
    %
    % 1. `pagebackref=true` adds ‘backlink’ text to the end of each item in the bibliography, as a list of page numbers
    % 2. `bookmarks=false` turns off Acrobat bookmarks
    %
    % CTAN: https://ctan.org/pkg/hyperref
    % Reference: https://en.wikibooks.org/wiki/LaTeX/Hyperlinks

    \usepackage[
        pagebackref=true,
        bookmarks=false
    ]{hyperref}

}{
    % Draft mode is off

    % ## Use hyperref – Extensive support for hypertext in LATEX

    \usepackage[
        bookmarks=false
    ]{hyperref}

}

%%%%%%%%%%%%%%%%%%%%%%%%%%%%%%%%%%%%%%%%%%%%%%%%%%%%%%%%%%%%%%%%%%%%%%%%%%%%%%%
% # Customize
%%%%%%%%%%%%%%%%%%%%%%%%%%%%%%%%%%%%%%%%%%%%%%%%%%%%%%%%%%%%%%%%%%%%%%%%%%%%%%%

\ifbool{draftmode}{
    % Draft mode is on

    % ## Customize hyperref
    %
    % Make hyperlinks easy to be spotted.

    \ifdef{\hypersetup}{
        % Package `hyperref` is used

        \hypersetup{
            % Colors the text of links and anchors
            colorlinks=true,
            % Color for normal internal links
            linkcolor=blue,
            % Color for bibliographical citations in text
            citecolor=red,
            % Color for linked URLs
            urlcolor=blue
        }

    }{
        % Package `hyperref` is not used
    }

}{
    % Draft mode is off
}
