# Supplementary material for: Reducing the Deployment-Time Inference Control Costs of Deep Reinforcement Learning Agents via an Asymmetric Architecture
Source: arXiv:2105.14471 source file (2021-05-30)
Supplement: Supplementary file 4 [file layout.tex]

% References:
% https://en.wikibooks.org/wiki/LaTeX/Page_Layout

%%%%%%%%%%%%%%%%%%%%%%%%%%%%%%%%%%%%%%%%%%%%%%%%%%%%%%%%%%%%%%%%%%%%%%%%%%%%%%%
% # Use Packages
%%%%%%%%%%%%%%%%%%%%%%%%%%%%%%%%%%%%%%%%%%%%%%%%%%%%%%%%%%%%%%%%%%%%%%%%%%%%%%%

% ## geometry – Flexible and complete interface to document dimensions
%
% This package is used to adjust page layout.
%
% ### Usage
%
% Use the command `\geometry{<options>}`. Available options are:
% 1. `hscale=<float>`: Set ratio of width of total body to paper width (Default: `0.7`)
% 2. `vscale=<float>`: Set ratio of height of total body to paper height (Default: `0.7`)
% 3. `footskip=<length>`: Set spacing between baseline of last line of text and baseline of footer
% 4. `footnotesep=<length>`: Set spacing between the bottom of text body and the top of footnote text
%
% ### Examples
%
% To make text more occupied on a page, write:
% ```latex
% \geometry{
%     hscale=0.75,
%     vscale=0.75
% }
% ```
%
% CTAN: https://ctan.org/pkg/geometry

% \usepackage{geometry}

%------------------------------------------------------------------------------

% ## multicol – Intermix single and multiple columns
%
% This package defines an environment which typesets text in multiple columns.
%
% ### Examples
%
% ```latex
% \begin{multicols}{2}
% [
% This sentence will show in one column.
% ]
% This sentence will show in two columns. This sentence will show in two columns. This sentence will show in two columns.
% \end{multicols}
% ```
%
% CTAN: https://ctan.org/pkg/multicol
% References:
% https://www.overleaf.com/learn/latex/Multiple_columns

\usepackage{multicol}

%%%%%%%%%%%%%%%%%%%%%%%%%%%%%%%%%%%%%%%%%%%%%%%%%%%%%%%%%%%%%%%%%%%%%%%%%%%%%%%
% # Customize
%%%%%%%%%%%%%%%%%%%%%%%%%%%%%%%%%%%%%%%%%%%%%%%%%%%%%%%%%%%%%%%%%%%%%%%%%%%%%%%

% ## Customize page number

% Check whether the draft mode is on
\ifbool{draftmode}{
    % Draft mode is on

    % Show the page numbers at the bottom of every page
    \pagestyle{plain}
}{
    % Draft mode is off
}

% ## Customize geometry
%
% Change ratio of body text to paper size.
% It is not recommended to adjust these spacing. It is wiser to reduce words.

\ifdef{\geometry}{
    % Package `geometry` is used

    % \geometry{
    %     % Ratio of width of total body to paper width
    %     hscale=0.75,
    %     % Ratio of height of total body to paper height
    %     vscale=0.75
    % }

}{
    % Package `geometry` is not used
}
