# Supplementary material for: Reducing the Deployment-Time Inference Control Costs of Deep Reinforcement Learning Agents via an Asymmetric Architecture
Source: arXiv:2105.14471 source file (2021-05-30)
Supplement: Supplementary file 5 [file sections.tex]

%%%%%%%%%%%%%%%%%%%%%%%%%%%%%%%%%%%%%%%%%%%%%%%%%%%%%%%%%%%%%%%%%%%%%%%%%%%%%%%
% # Use Packages
%%%%%%%%%%%%%%%%%%%%%%%%%%%%%%%%%%%%%%%%%%%%%%%%%%%%%%%%%%%%%%%%%%%%%%%%%%%%%%%

% ## titlesec – Select alternative section titles
%
% This package is used for adjusting spacing before and after section titles.
%
% ### Usage
%
% To adjust the vertical spacing before and after the section titles, write:
% ```latex
% \titlespacing{<command>}{<left>}{<before-sep>}{<after-sep>}
% ```
% Available options are:
% 1. `command`: Command to be adjusted
% 2. `left`: Horizontal spacing on the left side of the command
% 3. `before-sep`: Vertical spacing before the command
% 4. `after-sep`: Vertical spacing after the command
%
% For more advanced usage, please see the documentation on CTAN.
%
% ### Examples
%
% To have specific spacing, set the values directly:
% ```latex
% \titlespacing{\section}{0pt}{3.5ex plus 1ex minus .2ex}{2.3ex plus .2ex}
% ```
%
% To have relative spacing to default spacing, set the multiplication:
% ```latex
% \titlespacing{\section}{0pt}{*.5}{*.5}
% ```
%
% CTAN: https://ctan.org/pkg/titlesec

% \usepackage{titlesec}

%%%%%%%%%%%%%%%%%%%%%%%%%%%%%%%%%%%%%%%%%%%%%%%%%%%%%%%%%%%%%%%%%%%%%%%%%%%%%%%
% # Customize
%%%%%%%%%%%%%%%%%%%%%%%%%%%%%%%%%%%%%%%%%%%%%%%%%%%%%%%%%%%%%%%%%%%%%%%%%%%%%%%

% ## Customize titlesec
%
% Change vertical spacing before and after section titles.
% It is not recommended to adjust these spacing. It is wiser to reduce words.

\ifdef{\titlespacing}{
    % Package `titlesec` is used

    % % section
    % \titlespacing{\section}{0pt}{*.5}{*.5}
    % % subsection
    % \titlespacing{\subsection}{0pt}{*.5}{*.5}
    % % subsubsection
    % \titlespacing{\subsubsection}{0pt}{*.5}{*.5}
    % % paragraph
    % \titlespacing{\paragraph}{0pt}{*.5}{*.5}
    % % subparagraph
    % \titlespacing{\subparagraph}{0pt}{*.5}{*.5}

}{
    % Package `titlesec` is not used
}
