# Supplementary material for: Reducing the Deployment-Time Inference Control Costs of Deep Reinforcement Learning Agents via an Asymmetric Architecture
Source: arXiv:2105.14471 source file (2021-05-30)
Supplement: Supplementary file 6 [file algorithms.tex]

\usepackage{algorithm}

\usepackage[
]{algpseudocode}
