# Supplementary material for: Reducing the Deployment-Time Inference Control Costs of Deep Reinforcement Learning Agents via an Asymmetric Architecture
Source: arXiv:2105.14471 source file (2021-05-30)
Supplement: Supplementary file 7 [file annotations.tex]

%%%%%%%%%%%%%%%%%%%%%%%%%%%%%%%%%%%%%%%%%%%%%%%%%%%%%%%%%%%%%%%%%%%%%%%%%%%%%%%
% # Use Packages
%%%%%%%%%%%%%%%%%%%%%%%%%%%%%%%%%%%%%%%%%%%%%%%%%%%%%%%%%%%%%%%%%%%%%%%%%%%%%%%

% ## FiXme - Collaborative annotation tool for LATEX
%
% This package allows you to annotate the document.
%
% ### Usage
%
% You can use the following commands to add inline annotations:
% ```latex
% \fxnote{<note>}
% \fxwarning{<note>}
% \fxerror{<note>}
% \fxfatal{<note>}
%
% \fxnote*{<note>}{<text>}
% \fxwarning*{<note>}{<text>}
% \fxerror*{<note>}{<text>}
% \fxfatal*{<note>}{<text>}
% ```
%
% ### Examples
%
% Add the following line in the document:
% ```latex
% \fxwarning{should add reference here}
% \fxerror{the reference is wrong}
% \fxnote*{move to section 2}{We present the ﬁrst deep learning model...}
% \fxerror*{please add figure}{Figure ? provides sample screenshots...}
% ```
%
% CTAN: https://ctan.org/pkg/fixme

\usepackage{fixme}

%%%%%%%%%%%%%%%%%%%%%%%%%%%%%%%%%%%%%%%%%%%%%%%%%%%%%%%%%%%%%%%%%%%%%%%%%%%%%%%
% # Customize
%%%%%%%%%%%%%%%%%%%%%%%%%%%%%%%%%%%%%%%%%%%%%%%%%%%%%%%%%%%%%%%%%%%%%%%%%%%%%%%

% Check whether the draft mode is on
\ifbool{draftmode}{
    % Draft mode is on

    % ## Customize fixme
    %
    % Show FiXme annotations inline and with color.

    \ifdef{\fxsetup}{
        % Package `fixme` is used

        \fxsetup{
            status=draft,
            layout=inline,
            author=,
            theme=color
        }

    }{
        % Package `fixme` is not used
    }

}{
    % Draft mode is off

    % ## Customize fixme
    %
    % Hide FiXme annotations.

    \ifdef{\fxsetup}{
        % Package `fixme` is used

        \fxsetup{
            status=final
        }

    }{
        % Package `fixme` is not used
    }

}
