# Supplementary material for: Reducing the Deployment-Time Inference Control Costs of Deep Reinforcement Learning Agents via an Asymmetric Architecture
Source: arXiv:2105.14471 source file (2021-05-30)
Supplement: Supplementary file 8 [file appendix.tex]

%%%%%%%%%%%%%%%%%%%%%%%%%%%%%%%%%%%%%%%%%%%%%%%%%%%%%%%%%%%%%%%%%%%%%%%%%%%%%%%
% # Use Packages
%%%%%%%%%%%%%%%%%%%%%%%%%%%%%%%%%%%%%%%%%%%%%%%%%%%%%%%%%%%%%%%%%%%%%%%%%%%%%%%

% ## appendix – Extra control of appendices
%
% This package provides various ways of formatting the titles of appendices.
%
% ### Usage
%
% Write the appendix content inside the `appendices` environment:
% ```latex
% \begin{appendices}
% <Appendix Content>
% \end{appendices}
% ```
% You can customize the appendix environment:
% 1. Customize the appendix title (Default is "Appendices"):
%   ```latex
%   \renewcommand{\appendixpagename}{Supplementary Material}
%   ```
% 2. Add the appendix title with the command `\appendixpage`.
% 3. Change the section numbering format (Default is `\renewcommand{\thesection}{\Alph{section}}`):
%   ```latex
%   \renewcommand{\thesection}{S.\arabic{section}}
%   ```
%
% ### Examples
%
% To begin the appendix section, add the following at the end of document:
% ```latex
% \begin{appendices}
% \section{Appendix 1}
% Dummy text.
% \end{appendices}
% ```
%
% CTAN: https://ctan.org/pkg/appendix

\usepackage{appendix}
