# Supplementary material for: Reducing the Deployment-Time Inference Control Costs of Deep Reinforcement Learning Agents via an Asymmetric Architecture
Source: arXiv:2105.14471 source file (2021-05-30)
Supplement: Supplementary file 9 [file bibliography.tex]

\usepackage[
]{natbib}

%%%%%%%%%%%%%%%%%%%%%%%%%%%%%%%%%%%%%%%%%%%%%%%%%%%%%%%%%%%%%%%%%%%%%%%%%%%%%%%
% # Customize
%%%%%%%%%%%%%%%%%%%%%%%%%%%%%%%%%%%%%%%%%%%%%%%%%%%%%%%%%%%%%%%%%%%%%%%%%%%%%%%

% ## Customize biblatex
%
% 1. Import bibtex data file
% 2. Set preamble options

\ifdef{\addbibresource}{
    % Package `biblatex` is used

    % Replace `references.bib` with proper file
    \addbibresource{references.bib}
    % Set preamble options
    \ExecuteBibliographyOptions{
    }

}{
    % Package `biblatex` is not used
}

%------------------------------------------------------------------------------

% ## Customize natbib
%
% Change citation punctuation.

\ifdef{\setcitestyle}{
    % Package `natbib` is used

    % \setcitestyle{}

}{
    % Package `natbib` is not used
}
