# Supplementary material for: Reducing the Deployment-Time Inference Control Costs of Deep Reinforcement Learning Agents via an Asymmetric Architecture
Source: arXiv:2105.14471 source file (2021-05-30)
Supplement: Supplementary file 10 [file characters.tex]

% References:
% https://en.wikibooks.org/wiki/LaTeX/Special_Characters

%%%%%%%%%%%%%%%%%%%%%%%%%%%%%%%%%%%%%%%%%%%%%%%%%%%%%%%%%%%%%%%%%%%%%%%%%%%%%%%
% # Use Packages
%%%%%%%%%%%%%%%%%%%%%%%%%%%%%%%%%%%%%%%%%%%%%%%%%%%%%%%%%%%%%%%%%%%%%%%%%%%%%%%

% ## microtype – Subliminal refinements towards typographical perfection
%
% This package greatly improves general appearance of the text.
%
% Using this package will make a single line more likely to contain more words, thus reducing the overall space a paragraph occupies.
%
% CTAN: https://ctan.org/pkg/microtype
% Reference: http://www.khirevich.com/latex/microtype/

\usepackage{microtype}

\usepackage{siunitx}

%------------------------------------------------------------------------------

% ## textcomp – LATEX support for the Text Companion fonts
%
% This package provides many text symbols.
%
% ### Usage
%
% Find symbols in references.
%
% ### Examples
%
% ```latex
% a \textminus b
% ```
%
% CTAN: https://ctan.org/pkg/textcomp
% References:
% 1. http://detexify.kirelabs.org/classify.html
% 2. http://gcp.fcaglp.unlp.edu.ar/_media/integrantes:psantamaria:latex:textcomp.pdf
% 3. https://ctan.org/pkg/comprehensive

\usepackage{textcomp}

%------------------------------------------------------------------------------

% ## textgreek – Upright greek letters in text
%
% This package provides upright Greek letters in text.
%
% ### Usage
%
% Find symbols in references.
%
% ### Examples
%
% ```latex
% \textbeta-decay
% ```
%
% CTAN: https://ctan.org/pkg/textgreek
% References:
% 1. http://detexify.kirelabs.org/classify.html
% 2. https://ctan.org/pkg/comprehensive

\usepackage{textgreek}
