# Supplementary material for: Reducing the Deployment-Time Inference Control Costs of Deep Reinforcement Learning Agents via an Asymmetric Architecture
Source: arXiv:2105.14471 source file (2021-05-30)
Supplement: Supplementary file 11 [file lists.tex]

% References:
% https://en.wikibooks.org/wiki/LaTeX/List_Structures

%%%%%%%%%%%%%%%%%%%%%%%%%%%%%%%%%%%%%%%%%%%%%%%%%%%%%%%%%%%%%%%%%%%%%%%%%%%%%%%
% # Use Packages
%%%%%%%%%%%%%%%%%%%%%%%%%%%%%%%%%%%%%%%%%%%%%%%%%%%%%%%%%%%%%%%%%%%%%%%%%%%%%%%

% ## enumitem – Control layout of itemize, enumerate, description
%
% This package is used for reducing vertical spacing between enumerate items.
%
% CTAN: https://ctan.org/pkg/enumitem

\usepackage{enumitem}

%%%%%%%%%%%%%%%%%%%%%%%%%%%%%%%%%%%%%%%%%%%%%%%%%%%%%%%%%%%%%%%%%%%%%%%%%%%%%%%
% # Customize
%%%%%%%%%%%%%%%%%%%%%%%%%%%%%%%%%%%%%%%%%%%%%%%%%%%%%%%%%%%%%%%%%%%%%%%%%%%%%%%

% ## Customize enumitem
%
% Change vertical spacing between items.

\ifdef{\setlist}{
    % Package `enumitem` is used

    % \setlist{
    %     % Vertical spacing before and after the item area
    %     topsep=0ex,
    %     % Vertical spacing before and after the item area if there are blank lines
    %     partopsep=0ex,
    %     % Vertical spacing between two paragraphs
    %     parsep=0ex,
    %     % Vertical spacing between two items
    %     itemsep=0.5ex
    % }

}{
    % Package `enumitem` is not used
}
