# Supplementary material for: Reducing the Deployment-Time Inference Control Costs of Deep Reinforcement Learning Agents via an Asymmetric Architecture
Source: arXiv:2105.14471 source file (2021-05-30)
Supplement: Supplementary file 12 [file mathematics.tex]

% References:
% https://en.wikibooks.org/wiki/LaTeX/Mathematics

%%%%%%%%%%%%%%%%%%%%%%%%%%%%%%%%%%%%%%%%%%%%%%%%%%%%%%%%%%%%%%%%%%%%%%%%%%%%%%%
% # Use Packages
%%%%%%%%%%%%%%%%%%%%%%%%%%%%%%%%%%%%%%%%%%%%%%%%%%%%%%%%%%%%%%%%%%%%%%%%%%%%%%%

% ## amsmath – AMS mathematical facilities for LATEX
%
% This package provides miscellaneous enhancements for improving the information structure and printed output of documents containing mathematical formulas.
%
% CTAN: https://ctan.org/pkg/amsmath
% Reference: https://tex.stackexchange.com/a/32102

\usepackage{amsmath}

%------------------------------------------------------------------------------

% ## amssymb
%
% This package internally loads "amsfonts", which provides extended set of fonts for use in mathematics.
%
% Reference: https://tex.stackexchange.com/a/32102
% See also: https://ctan.org/pkg/amsfonts

\usepackage{amssymb}

%------------------------------------------------------------------------------

% ## amsthm – Typesetting theorems (AMS style)
%
% This package helps to define theorem-like structures.
%
% CTAN: https://ctan.org/pkg/amsthm
% Reference: https://tex.stackexchange.com/a/32102

\usepackage{amsthm}

%------------------------------------------------------------------------------

% ## bbm – "Blackboard-style" cm fonts
%
% This package provides blackboard variants of Computer Modern fonts.
%
% ### Usage
%
% This package provides the following commands:
% 1. `\mathbbm{<text>}`: Blackboard text in Roman font.
% 2. `\mathbbmss{<text>}`: Blackboard text in Sans Serif font.
% 3. `\mathbbmtt{<text>}`: Blackboard text in Typewriter font.
%
% You can also put `\mathbold` before the above commands to use bold letters.
%
% ### Examples
%
% ```latex
% \begin{enumerate}
%     \item \texttt{\textbackslash mathbbm}: $\mathbbm{N},\mathbbm{i},\mathbbm{1}$
%     \item \texttt{\textbackslash mathbbmss}: $\mathbbmss{N},\mathbbmss{i},\mathbbmss{1}$
%     \item \texttt{\textbackslash mathbbmtt}: $\mathbbmtt{N},\mathbbmtt{i},\mathbbmtt{1}$
% \end{enumerate}
% ```
%
% CTAN: https://ctan.org/pkg/bbm
% See also: https://ctan.org/pkg/bbm-macros

\usepackage{bbm}

%------------------------------------------------------------------------------

% ## mathrsfs – Support for using RSFS fonts in maths
%
% This package provides mathematical script letters.
%
% ### Examples
%
% ```latex
% \mathscr{ABCDEFGHIJKLMNOPQRSTUVWXYZ}
% ```
%
% CTAN: https://ctan.org/pkg/mathrsfs
% References:
% https://www.stat.colostate.edu/~vollmer/pdfs/typesetting-script.pdf

\usepackage{mathrsfs}

\usepackage{mathtools}

%------------------------------------------------------------------------------

% ## xfrac – Split-level fractions in LATEX2ε*
%
% This package allows the user to typeset fractions in the form ‘n/d’.
%
% ### Usage
%
% To insert fraction in the form "n/d", write:
% ```latex
% \sfrac{<num>}{<denom>}
% ```
%
% ### Examples
%
% To insert the fraction "1/2", write:
% ```latex
% $\sfrac{1}{2}$
% ```
%
% CTAN: https://ctan.org/pkg/xfrac

\usepackage{xfrac}
