# Supplementary material for: Reducing the Deployment-Time Inference Control Costs of Deep Reinforcement Learning Agents via an Asymmetric Architecture
Source: arXiv:2105.14471 source file (2021-05-30)
Supplement: Supplementary file 13 [file project.tex]

% # Customization for Project
%
% This file adds customization only for this project.

% ## Define commonly written texts

% ### Algorithm Names

% A2C

% Curiosity

% PPO

% ### Game Environments

% Atari (Full)

% Doom (Full)

% Doom (Abbreviation)

% ### Game Names

% Atari

% Doom

% ### Macros

% Discovered macro

% ### Method Names

% Human

% Random

% Repeat

% ### Pseudo-code

% Action space

% DRL Algorithm

% Environment

% State space

% ## Define commonly written algorithm commands

% For writing one line if-then pseudocode.
% Available command: \IfThen{<if>}{<then>}
\algnewcommand{\IfThen}[2]{\State \algorithmicif\ #1\ \algorithmicthen\ #2}

% ## Define commonly written 
