# Supplementary material for: Reducing the Deployment-Time Inference Control Costs of Deep Reinforcement Learning Agents via an Asymmetric Architecture
Source: arXiv:2105.14471 source file (2021-05-30)
Supplement: Supplementary file 14 [file spacing.tex]

%%%%%%%%%%%%%%%%%%%%%%%%%%%%%%%%%%%%%%%%%%%%%%%%%%%%%%%%%%%%%%%%%%%%%%%%%%%%%%%
% # Use Packages
%%%%%%%%%%%%%%%%%%%%%%%%%%%%%%%%%%%%%%%%%%%%%%%%%%%%%%%%%%%%%%%%%%%%%%%%%%%%%%%

% ## setspace – Set space between lines
%
% This package allows you to adjust the spacing between lines in a document.
%
% ### Usage
%
% Use the environment `\begin{spacing}{<stretch>}` to surround the content to be stretched. Smaller `<stretch>` will have less vertical spacing. Default `<stretch>` is `1`.
%
% ### Examples
%
% Reduce the vertical spacing between equations:
% ```latex
% \begin{spacing}{0.5}
%     \begin{equation}
%         x=y
%     \end{equation}
%     \begin{equation}
%         x=y
%     \end{equation}
% \end{spacing}
% ```
%
% CTAN: https://ctan.org/pkg/setspace
% Reference: https://texblog.org/2011/09/30/quick-note-on-line-spacing/

\usepackage{setspace}
