# Supplementary material for: Reducing the Deployment-Time Inference Control Costs of Deep Reinforcement Learning Agents via an Asymmetric Architecture
Source: arXiv:2105.14471 source file (2021-05-30)
Supplement: Supplementary file 15 [file tables.tex]

% References:
% https://en.wikibooks.org/wiki/LaTeX/Tables

%%%%%%%%%%%%%%%%%%%%%%%%%%%%%%%%%%%%%%%%%%%%%%%%%%%%%%%%%%%%%%%%%%%%%%%%%%%%%%%
% # Use Packages
%%%%%%%%%%%%%%%%%%%%%%%%%%%%%%%%%%%%%%%%%%%%%%%%%%%%%%%%%%%%%%%%%%%%%%%%%%%%%%%

% ## array – Extending the array and tabular environments
%
% This package improves the appearance of tables.
%
% ### Usage
%
% The first `\hline` should be replaced with `\firsthline` and the last `\hline` should be replaced with `\lasthline` to fix the aligning problem with texts if you switch from "tabular" to this package.
%
% ### Examples
%
% ```latex
% \begin{table}[t]
%     \centering
%     \begin{tabular}{llr}
%         \firsthline
%         \multicolumn{2}{c}{Item} \\
%         \cline{1-2}
%         Animal    & Description & Price (\$) \\
%         \hline
%         Gnat      & per gram    & 13.65      \\
%                   & each        & 0.01       \\
%         Gnu       & stuffed     & 92.50      \\
%         Emu       & stuffed     & 33.33      \\
%         Armadillo & frozen      & 8.99       \\
%         \lasthline
%     \end{tabular}
%     \caption{A table.}
%     \label{tab:table}
% \end{table}
% ```
%
% CTAN: https://ctan.org/pkg/array
% Reference: https://en.wikibooks.org/wiki/LaTeX/Tables

\usepackage{array}

%------------------------------------------------------------------------------

% ## booktabs – Publication quality tables in LATEX
%
% This package improves the appearance of tables.
%
% ### Usage
%
% This package provides several commands to replace `\hline` (with `\toprule`, `\midrule` and `\bottomrule`) and `\cline` (with `\cmidrule`) in "tabular" package:
% 1. `\toprule[<wd>]`: Producing a thick top line
% 2. `\midrule[<wd>]`: Producing a light dividing line
% 3. `\bottomrule[<wd>]`: Producing a thick bottom line
% 4. `\cmidrule[<wd>]{a-b}`: Producing a subline to extend over only some columns
% `<wd>` is the thickness of the line, it is not recommended to specify it for each line. It is more recommended to change the lengths `\lightrulewidth` (for `\midrule`) and `\heavyrulewidth` (for `\toprule` and `\bottomrule`) globally. If you want more than one `\cmidrule`, add a `\morecmidrules` between two `\cmidrule`.
%
% ### Examples
%
% ```latex
% \begin{table}[t]
%     \centering
%     \begin{tabular}{llr}
%         \toprule
%         \multicolumn{2}{c}{Item} \\
%         \cmidrule{1-2}
%         Animal    & Description & Price (\$) \\
%         \midrule
%         Gnat      & per gram    & 13.65      \\
%                   & each        & 0.01       \\
%         Gnu       & stuffed     & 92.50      \\
%         Emu       & stuffed     & 33.33      \\
%         Armadillo & frozen      & 8.99       \\
%         \bottomrule
%     \end{tabular}
%     \caption{A table.}
%     \label{tab:table}
% \end{table}
% ```
%
% CTAN: https://ctan.org/pkg/booktabs
% Reference: https://en.wikibooks.org/wiki/LaTeX/Tables

\usepackage{booktabs}

%------------------------------------------------------------------------------

% ## multirow – Create tabular cells spanning multiple rows
%
% This package is used for creating texts spanning multiple rows.
%
% ### Usage
%
% To create texts spanning multiple rows, use the command:
% ```latex
% \multirow[<vpos>]{<nrows>}{<width>}[<vmove>]{<text>}
% ```
% Available options are:
% 1. `<vpos>`: Vertical positioning of text
%   1. `c`: Vertically centered text (default)
%   2. 't': Top-aligned text
%   3. `b`: Bottom-aligned text
% 2. `<nrows>`: Number of rows to span
% 3. `<width>: Text width to be set
%   1. `*`: Use text parameter's natural width
%   2. `=`: Use specified width of column set by `\multirow`
% 4. `<vmove>`: The height of text to be raised. Use positive value to raise the text, or negative value to lower the text
% 5. `<text>`: Text to be inserted
%
% ### Examples
%
% ```latex
% \begin{table}[t]
%     \centering
%     \begin{tabular}{llr}
%         \hline
%         \multicolumn{2}{c}{Item} \\
%         \cline{1-2}
%         Animal                  & Description & Price (\$)          \\
%         \hline
%         \multirow{2}{*}{Gnat*}  & per gram                  & 13.65 \\
%                                 & each                      & 0.01  \\
%         Gnu                     & \multirow{2}{*}{stuffed*} & 92.50 \\
%         Emu                     &                           & 33.33 \\
%         Armadillo & frozen      & 8.99                              \\
%         \hline
%     \end{tabular}
%     \caption{A table.}
%     \label{tab:table}
% \end{table}
% ```
%
% CTAN: https://ctan.org/pkg/multirow

\usepackage{multirow}

\usepackage{tabu}

%------------------------------------------------------------------------------

% ## tabularx – Tabulars with adjustable-width columns
%
% This package provides more flexibility to adjust widths of tables.
%
% ### Usage
%
% Use the environment `\begin{tabularx}{<width>}{<preamble>}`. Available options are:
% 1. `width`: Desired width of table.
% 2. `preamble`: You can add the column specifier `X` to have the columns stretched to make the table as wide as specified by `width`
%
% ### Examples
%
% You can add the following column types to have different alignments:
% ```latex
% % Left-aligned
% \newcolumntype{L}{>{\raggedright\arraybackslash}X}
% % Right-aligned
% \newcolumntype{R}{>{\raggedleft\arraybackslash}X}
% % Center-aligned
% \newcolumntype{C}{>{\centering\arraybackslash}X}
% ```
% For example:
% ```latex
% \begin{table}[t]
%     \centering
%     \begin{tabularx}{0.9\linewidth}{|L|C|R|X|}
%         \hline
%         label 1     & label 2   & label 3     & label 4     \\
%         \hline
%         long item 1 & item 2    & long item 3 & long item 4 \\
%         \hline
%     \end{tabularx}
%     \caption{A table.}
%     \label{tab:table}
% \end{table}
% ```
%
% CTAN: https://ctan.org/pkg/tabularx
% Reference: https://en.wikibooks.org/wiki/LaTeX/Tables

\usepackage{tabularx}

%------------------------------------------------------------------------------

% ## tabulary – Tabular with variable width columns balanced
%
% This package provides more flexibility to adjust widths of tables.
%
% This package tries to balance the column widths so that each column has at least its natural width, without exceeding the maximum length. The problem with "tabularx" is that it leaves much blank if your cells are almost empty.
%
% ### Usage
%
% Use the environment `\begin{tabulary}{<length>}{<pream>}`. Available options are:
% 1. `length`: Desired width of table.
% 2. `pream`: You can add following column specifiers:
%   1. `L`: Left-justified balanced column
%   2. `C`: Center-justified balanced column
%   3. `R`: Right-justified balanced column
%   4. `J`: Normally-justified balanced column
%
% ### Examples
%
% ```latex
% \begin{table}[t]
%     \centering
%     \begin{tabulary}{0.9\linewidth}{|L|C|R|J|}
%         \hline
%         label 1     & label 2   & label 3     & label 4     \\
%         \hline
%         long item 1 & item 2    & long item 3 & long item 4 \\
%         \hline
%     \end{tabulary}
%     \caption{A table.}
%     \label{tab:table}
% \end{table}
% ```
%
% CTAN: https://ctan.org/pkg/tabulary
% Reference: https://en.wikibooks.org/wiki/LaTeX/Tables

\usepackage{tabulary}

%%%%%%%%%%%%%%%%%%%%%%%%%%%%%%%%%%%%%%%%%%%%%%%%%%%%%%%%%%%%%%%%%%%%%%%%%%%%%%%
% # Customize
%%%%%%%%%%%%%%%%%%%%%%%%%%%%%%%%%%%%%%%%%%%%%%%%%%%%%%%%%%%%%%%%%%%%%%%%%%%%%%%

% ## Customize booktabs
%
% 1. Change line widths
% 2. Change vertical spacing before and after lines

\ifdef{\heavyrulewidth}{
    % % Package `booktabs` is used

    % % Change line width for `\toprule` and `\bottomrule`
    % \setlength{\heavyrulewidth}{.08em}
    % % Change line width for `\midrule`
    % \setlength{\lightrulewidth}{.05em}
    % % Change line width for `cmidrule`
    % \setlength{\cmidrulewidth}{.03em}
    % % Change vertical spacing before lines except `\toprule`
    % \setlength{\aboverulesep}{0ex}
    % % Change vertical spacing after lines except `\bottomrule`
    % \setlength{\belowrulesep}{0ex}
    % % Change vertical spacing between two `\cmidrule`
    % \setlength{\cmidrulesep}{\doublerulesep}

}{
    % Package `booktabs` is not used
}

%------------------------------------------------------------------------------

% ## Customize tabu
%
% Change vertical spacing between the cell content and the cell border.

\ifcsdef{tabu}{
    % % Package `tabu` is used

    % % Set the minimal vertical space allowed between the cell content and the cell border
    % \setlength{\tabulinesep}{3pt}

}{
    % Package `tabu` is not used
}
